# Supplementary material for: Computer-Aided Data Mining: Automating a Novel Knowledge Discovery and Data Mining Process Model for Metabolomics
Source: arXiv:1907.04318 source file (2019-07-09)
Supplement: Supplementary file 1 [file dataminingobjectives.pdf]

```
<?xml version="1.0" encoding="UTF-8" standalone="true"?>
<dataMiningObjective xsi:noNamespaceSchemaLocation="" version="1"
xmlns:xsi="http://www.w3.org/2001/XMLSchema-instance">
    <dateTime>Tue Mar 13 20:14:00 GMT 2012</dateTime>
    <description>Classifying the samples into the area of metabolism classed which are linked to the plant
      genotypes.</description>
    <location>E:\PhD\PhD\PhDThesis\PhDApplication\HiMet9IP_Application\HiMet9IP_11\Process\Iteration 1
      \Phases\1- Objectives Definition\Iteration 1\Delivery</location>
  - <successCriteria>
        <description>This percentage should be between 50% and 99%</description>
      - <expectedOutcomes>
            <resultsList/>
          - <resultsList>
                <measure measureType="QUANTITATIVE" maximum="100.0" minimum="0.0"
                  unit="Prediction Accuracy" xsi:type="quantitativeMeasure"/>
                <outcome/>
            </resultsList>
          - <resultsList>
                <measure measureType="QUANTITATIVE" maximum="100.0" minimum="0.0"
                  unit="Classification Precision" xsi:type="quantitativeMeasure"/>
                <outcome/>
            </resultsList>
        </expectedOutcomes>
    </successCriteria>
    <approach>HYPOTHESIS_DRIVEN</approach>
  - <traceability>
      - <externalSourcesList xsi:type="externalSource" sourceType="ExternalSource">
            <description>PhD Thesis</description>
            <url>file:/E:/PhD/PhD/PhDThesis/PhDThesisWriting/PhDThesisLatex/PhDLatex/PhDThesis.pdf</url>
        </externalSourcesList>
      - <externalSourcesList xsi:type="externalSource" sourceType="ExternalSource">
            <description>Maria Likata Presentation about the acquired data in HiMet Project</description>
            <url>file:/E:/PhD/PhD/PhDThesis/PhDApplication/Application_Data/Plant_York_LC-
              MS_TargetAnalisis/Description/maria1.pdf</url>
        </externalSourcesList>
      - <externalSourcesList xsi:type="externalSource" sourceType="ExternalSource">
            <description>lynn Presentation about the experimental design of HiMet Project</description>
            <url>file:/E:/PhD/PhD/PhDThesis/PhDApplication/Application_Data/Plant_York_LC-
              MS_TargetAnalisis/Description/lynne.pdf</url>
        </externalSourcesList>
      - <externalSourcesList xsi:type="externalSource" sourceType="ExternalSource">
            <description>This paper was based on HiMet project, where the data was acquired. Scott, I. M., C. P.
              Vermeer, et al. (2010). "Enhancement of Plant Metabolite Fingerprinting by Machine Learning."
              Plant Physiology 153(4): 1506-1520.</description>
            <url>http://www.plantphysiol.org/content/153/4/1506.abstract</url>
        </externalSourcesList>
      - <internalSourcesList xsi:type="internalSource" sourceType="InternalSource">
            <sourceElementPath> [Process] -> [Inputs] -> Aims of Study</sourceElementPath>
        </internalSourcesList>
    </traceability>
  - <measurability>
        <quantitativeMeasuresList measureType="QUANTITATIVE" maximum="100.0" minimum="0.0"
          unit="Prediction Accuracy" xsi:type="quantitativeMeasure"/>
        <quantitativeMeasuresList measureType="QUANTITATIVE" maximum="100.0" minimum="0.0"
          unit="Classification Precision" xsi:type="quantitativeMeasure"/>
    </measurability>
```

```
- <feasibility>
  - <requiredResources>
    - <resourcesList xsi:type="resource" quantiy="1.0" cost="750.0" resourceType="HARDWARE"
        description="Labtop">
      - <requirements>
        - <requirementsList>
              <requirementsList xsi:type="resource" quantiy="1.0" cost="250.0"
                 resourceType="SOFTWARE" description="R Package"/>
              <requirementsList xsi:type="resource" quantiy="1.0" cost="0.0"
                 resourceType="SOFTWARE" description="MikeTex"/>
              <requirementsList xsi:type="resource" quantiy="1.0" cost="300.0"
                 resourceType="SOFTWARE" description="windows 7.0"/>
              <requirementsList xsi:type="resource" quantiy="1.0" cost="250.0"
                 resourceType="SOFTWARE" description="MS Office "/>
          </requirementsList>
        </requirements>
      </resourcesList>
    </requiredResources>
     <requiredTime>7.0</requiredTime>
     <feasible>true</feasible>
  </feasibility>
- <acheivability>
     <dataSufficient>true</dataSufficient>
     <dataRelivent>true</dataRelivent>
     <acheivableWithData>true</acheivableWithData>
  </acheivability>
   <fulfilled>false</fulfilled>
   <finalSelection>false</finalSelection>
</dataMiningObjective>
```
