# Supplementary material for: Computer-Aided Data Mining: Automating a Novel Knowledge Discovery and Data Mining Process Model for Metabolomics
Source: arXiv:1907.04318 source file (2019-07-09)
Supplement: Supplementary file 2 [file phaseobjectives.pdf]

```
<?xml version="1.0" encoding="UTF-8" standalone="true"?>
<phase xsi:noNamespaceSchemaLocation="" version="1" id="1.4.1" name="Technique Selection" number="4"
xmlns:xsi="http://www.w3.org/2001/XMLSchema-instance">
    <dateTime>Tue Mar 13 12:23:44 GMT 2012</dateTime>
    <status>ACTIVE</status>
    <location>E:\PhD\PhD\PhDThesis\PhDApplication\HiMet9IP_Application/HiMet9IP_11/Process/Iteration
      1/Phases/4- Technique Selection/Iteration 1</location>
  + <preRequisites>
  - <objectives version="1">
        <dateTime>Wed Mar 21 18:10:38 GMT 2012</dateTime>
    - <objectivesList version="1" xsi:type="phaseObjective">
          <dateTime>Wed Mar 21 18:10:38 GMT 2012</dateTime>
          <objectiveType>FUNCTIONAL</objectiveType>
          <presetDescription>1. Selecting the data mining technique(s) that fulfil the defined process
            objectives and suit the targeted metabolomics data.</presetDescription>
          <fulfilled>false</fulfilled>
          <customisedDescription>1. Selecting the data mining technique(s) that fulfil the defined process
            objectives and suit the targeted metabolomics data.</customisedDescription>
          <customised>true</customised>
      </objectivesList>
    - <objectivesList version="1" xsi:type="phaseObjective">
          <dateTime>Wed Mar 21 18:10:38 GMT 2012</dateTime>
          <objectiveType>MANAGEMENT_RELATED</objectiveType>
          <presetDescription>2. The selected technique performance must be measurable in model
            evaluation.</presetDescription>
          <fulfilled>false</fulfilled>
          <customisedDescription>2. The selected technique performance must be measurable in model
            evaluation.</customisedDescription>
          <customised>true</customised>
      </objectivesList>
    - <objectivesList version="1" xsi:type="phaseObjective">
          <dateTime>Wed Mar 21 18:10:38 GMT 2012</dateTime>
          <objectiveType>FUNCTIONAL</objectiveType>
          <presetDescription>3. The selected technique must have the potential to achieve the defined
            process ob- jective.</presetDescription>
          <fulfilled>false</fulfilled>
          <customisedDescription>3. The selected technique must have the potential to achieve the
            defined process ob- jective.</customisedDescription>
          <customised>true</customised>
      </objectivesList>
    - <objectivesList version="1" xsi:type="phaseObjective">
          <dateTime>Wed Mar 21 18:10:38 GMT 2012</dateTime>
          <objectiveType>MANAGEMENT_RELATED</objectiveType>
          <presetDescription>4. The application of the selected technique must be feasible, and it must
            consider the process management constraints and available resources.</presetDescription>
          <fulfilled>false</fulfilled>
          <customisedDescription>4. The application of the selected technique must be feasible, and it
            must consider the process management constraints and available
            resources.</customisedDescription>
          <customised>true</customised>
      </objectivesList>
```

- <objectivesList version="**1**" xsi:type="**phaseObjective**">
<dateTime>Wed Mar 21 18:10:38 GMT 2012</dateTime>
<objectiveType>MANAGEMENT_RELATED</objectiveType>
<presetDescription>5. The selection procedures must be comprehensive and unbiased, and it must cover all possible data mining techniques (see section 3.4).</presetDescription>
<fulfilled>false</fulfilled>
<customisedDescription>5. The selection procedures must be comprehensive and unbiased, and it must cover all possible data mining techniques (see section 3.4).</customisedDescription>
<customised>true</customised>
</objectivesList>
- <objectivesList version="**1**" xsi:type="**phaseObjective**">
<dateTime>Wed Mar 21 18:10:38 GMT 2012</dateTime>
<objectiveType>FUNCTIONAL</objectiveType>
<presetDescription>6. The selection strategy must be flexible and adjustable and consider the selection of alternative techniques in the case of feedback or iteration.</presetDescription>
<fulfilled>false</fulfilled>
<customisedDescription>6. The selection strategy must be flexible and adjustable and consider the selection of alternative techniques in the case of feedback or iteration.</customisedDescription>
<customised>true</customised>
</objectivesList>
- <objectivesList version="**1**" xsi:type="**phaseObjective**">
<dateTime>Wed Mar 21 18:10:38 GMT 2012</dateTime>
<objectiveType>MANAGEMENT_RELATED</objectiveType>
<presetDescription>7. The selection of white-box data mining techniques must be encouraged over the selection of the black-box ones, as they allow more justification, reasoning, and explanation of the modelling results.</presetDescription>
<fulfilled>false</fulfilled>
<customisedDescription>7. The selection of white-box data mining techniques must be encouraged over the selection of the black-box ones, as they allow more justification, reasoning, and explanation of the modelling results.</customisedDescription>
<customised>true</customised>
</objectivesList>
- <objectivesList version="**1**" xsi:type="**phaseObjective**">
<dateTime>Wed Mar 21 18:10:38 GMT 2012</dateTime>
<objectiveType>MANAGEMENT_RELATED</objectiveType>
<presetDescription>8. The selection must consider the possibility of using more than one data mining technique.</presetDescription>
<fulfilled>false</fulfilled>
<customisedDescription>8. The selection must consider the possibility of using more than one data mining technique.</customisedDescription>
<customised>true</customised>
</objectivesList>
</objectives>
+ <planning version="**1**">
+ <performing version="**1**">
+ <reporting version="**1**">
+ <result version="**1**">
<actors/>
</phase>
