# Supplementary material for: Computer-Aided Data Mining: Automating a Novel Knowledge Discovery and Data Mining Process Model for Metabolomics
Source: arXiv:1907.04318 source file (2019-07-09)
Supplement: Supplementary file 3 [file planning.pdf]

```
<?xml version="1.0" encoding="UTF-8" standalone="true"?>
<phase xsi:noNamespaceSchemaLocation="" version="1" id="1.4.1" name="Technique Selection" number="4"
xmlns:xsi="http://www.w3.org/2001/XMLSchema-instance">
    <dateTime>Tue Mar 13 12:23:44 GMT 2012</dateTime>
    <status>ACTIVE</status>
    <location>E:\PhD\PhD\PhDThesis\PhDApplication\HiMet9IP_Application/HiMet9IP_11/Process/Iteration 1/Phases/4-
      Technique Selection/Iteration 1</location>
  + <preRequisites>
  + <objectives version="1">
  - <planning version="1">
      <dateTime>Wed Mar 21 18:10:38 GMT 2012</dateTime>
    - <planList version="1" xsi:type="plan">
        <dateTime>Wed Mar 21 18:10:38 GMT 2012</dateTime>
      + <presetPlanItem>
      - <customisedPlanItem>
          <description>1. Identify the suitable data mining approach to be used for model building, based on the
            type of the process objectives defined in phase 1 and in light of the discussion in section
            3.2.</description>
        - <subPlanList xsi:type="planItem">
            <description/>
            <optional>false</optional>
          </subPlanList>
          <optional>false</optional>
        </customisedPlanItem>
      + <planner>
      + <objectives version="1">
        <customised>true</customised>
        <performed>false</performed>
      </planList>
    - <planList version="1" xsi:type="plan">
        <dateTime>Wed Mar 21 18:10:38 GMT 2012</dateTime>
      + <presetPlanItem>
      - <customisedPlanItem>
          <description>2. Match the process objective to the data mining goals and tasks, which are illustrated in
            figure 3.2(see section 3.3).</description>
        - <subPlanList xsi:type="planItem">
            <description/>
            <optional>false</optional>
          </subPlanList>
          <optional>false</optional>
        </customisedPlanItem>
      + <planner>
      + <objectives version="1">
        <customised>true</customised>
        <performed>false</performed>
      </planList>
    - <planList version="1" xsi:type="plan">
        <dateTime>Wed Mar 21 18:10:38 GMT 2012</dateTime>
      + <presetPlanItem>
      - <customisedPlanItem>
          <description>3. Match the process objective to the available data mining techniques using the illustration
            in table 3.1), and taking into consideration the results of data exploration phase regarding the nature,
            quality, and potential of the targeted data.</description>
        - <subPlanList xsi:type="planItem">
            <description/>
            <optional>false</optional>
          </subPlanList>
          <optional>false</optional>
        </customisedPlanItem>
      + <planner>
      + <objectives version="1">
        <customised>true</customised>
        <performed>false</performed>
      </planList>
```

```
- <planList version="1" xsi:type="plan">
    <dateTime>Wed Mar 21 18:10:38 GMT 2012</dateTime>
  + <presetPlanItem>
  - <customisedPlanItem>
      <description>4. Based on the steps 1-3, select the data mining technique that would fulfil the defined
        objectives and suit the targeted data.</description>
    - <subPlanList xsi:type="planItem">
        <description/>
        <optional>false</optional>
      </subPlanList>
      <optional>false</optional>
    </customisedPlanItem>
  + <planner>
  + <objectives version="1">
    <customised>true</customised>
    <performed>false</performed>
  </planList>
- <planList version="1" xsi:type="plan">
    <dateTime>Wed Mar 21 18:10:38 GMT 2012</dateTime>
  + <presetPlanItem>
  - <customisedPlanItem>
      <description>5. Identify the resources, which are required for applying the selected technique, e.g.
        software , hardware, expertise, etc.</description>
    - <subPlanList xsi:type="planItem">
        <description/>
        <optional>false</optional>
      </subPlanList>
      <optional>false</optional>
    </customisedPlanItem>
  + <planner>
  + <objectives version="1">
    <customised>true</customised>
    <performed>false</performed>
  </planList>
- <planList version="1" xsi:type="plan">
    <dateTime>Wed Mar 21 18:10:38 GMT 2012</dateTime>
  + <presetPlanItem>
  - <customisedPlanItem>
      <description>6. Perform the following assessments on the candidate technique: (a) Assess the potential
        fulfilment of the defined process objectives by the candidate technique; (b) Assess the suitability of
        the candidate technique to the nature and quality of the data, as well as to its trends and expected
        patterns, based on the results of phase 3; (c) Assess the intense of the acclimatisation activities,
        which are required by the candidate technique; (d) Assess the availability of the resources required
        for applying the candidate technique; (e) Assess the feasibility of the application of the candidate
        technique; In the case of the candidate techniques failure in assessments in step 6, consider selecting
        an alternative technique by repeating the steps 4-6.</description>
    - <subPlanList xsi:type="planItem">
        <description/>
        <optional>false</optional>
      </subPlanList>
      <optional>false</optional>
    </customisedPlanItem>
  + <planner>
  + <objectives version="1">
    <customised>true</customised>
    <performed>false</performed>
  </planList>
- <planList version="1" xsi:type="plan">
    <dateTime>Wed Mar 21 18:10:38 GMT 2012</dateTime>
  + <presetPlanItem>
  - <customisedPlanItem>
      <description>7. Identify the performance measurements, which are applicable to the selected technique,
        e.g. accuracy, sensitivity, precision, specificity, etc.</description>
    - <subPlanList xsi:type="planItem">
```

<description/>
<optional>false</optional>
</subPlanList>
<optional>false</optional>
</customisedPlanItem>
+ <planner>
+ <objectives version="**1**">
<customised>true</customised>
<performed>false</performed>
</planList>
- <planList version="**1**" xsi:type="**plan**">
<dateTime>Wed Mar 21 18:10:38 GMT 2012</dateTime>
+ <presetPlanItem>
- <customisedPlanItem>
<description>8. Define the success criteria, based on the identify measurement.</description>
- <subPlanList xsi:type="**planItem**">
<description/>
<optional>false</optional>
</subPlanList>
<optional>false</optional>
</customisedPlanItem>
+ <planner>
+ <objectives version="**1**">
<customised>true</customised>
<performed>false</performed>
</planList>
- <planList version="**1**" xsi:type="**plan**">
<dateTime>Wed Mar 21 18:10:38 GMT 2012</dateTime>
+ <presetPlanItem>
- <customisedPlanItem>
<description>9. Define a mechanism for applying the selected modelling technique, considering its required resources identified in 5 and assessed in 6.</description>
- <subPlanList xsi:type="**planItem**">
<description/>
<optional>false</optional>
</subPlanList>
<optional>false</optional>
</customisedPlanItem>
+ <planner>
+ <objectives version="**1**">
<resources/>
<customised>true</customised>
<performed>false</performed>
</planList>
</planning>
+ <performing version="**1**">
+ <reporting version="**1**">
+ <result version="**1**">
<actors/>
</phase>
