# Supplementary material for: Computer-Aided Data Mining: Automating a Novel Knowledge Discovery and Data Mining Process Model for Metabolomics
Source: arXiv:1907.04318 source file (2019-07-09)
Supplement: Supplementary file 4 [file prerequisites.pdf]

```
<?xml version="1.0" encoding="UTF-8" standalone="true"?>
<phase xsi:noNamespaceSchemaLocation="" version="1" id="1.4.1" name="Technique Selection" number="4"
xmlns:xsi="http://www.w3.org/2001/XMLSchema-instance">
    <dateTime>Tue Mar 13 12:23:44 GMT 2012</dateTime>
    <status>ACTIVE</status>
    <location>E:\PhD\PhD\PhDThesis\PhDApplication\HiMet9IP_Application/HiMet9IP_11/Process/Iteration 1/Phases/4-
      Technique Selection/Iteration 1</location>
  - <preRequisites>
    - <preRequisitesList version="1" xsi:type="preRequisite">
        <dateTime>Wed Mar 21 18:10:38 GMT 2012</dateTime>
        <presetDescription>1. The pre-processed metabolomics dataset and its associated meta-data if available (see
          section 4.1).</presetDescription>
        <customisedDescription>1. The pre-processed metabolomics dataset and its associated meta-data if available (see
          section 4.1).</customisedDescription>
        <preRequisiteType>PROCESS_RELATED</preRequisiteType>
      - <sources>
        - <internalSourcesList xsi:type="internalSource" sourceType="InternalSource">
            <sourceElementPath> [Process] -> [Inputs] -> [Metabolomics Data] -> Data Set</sourceElementPath>
          </internalSourcesList>
        </sources>
        <required>false</required>
        <customised>true</customised>
      </preRequisitesList>
    - <preRequisitesList version="1" xsi:type="preRequisite">
        <dateTime>Wed Mar 21 18:10:38 GMT 2012</dateTime>
        <presetDescription>3. The data exploration report including the results of data investigation, understand- ing and
          prospecting.</presetDescription>
        <customisedDescription>3. The data exploration report including the results of data investigation, understand- ing
          and prospecting.</customisedDescription>
        <preRequisiteType>PROCESS_RELATED</preRequisiteType>
      - <sources>
        - <internalSourcesList xsi:type="internalSource" sourceType="InternalSource">
            <sourceElementPath> [Process] -> [Phases] -> [Data Exploration] -> Reporting</sourceElementPath>
          </internalSourcesList>
        </sources>
        <required>false</required>
        <customised>true</customised>
      </preRequisitesList>
    - <preRequisitesList version="1" xsi:type="preRequisite">
        <dateTime>Wed Mar 21 18:10:38 GMT 2012</dateTime>
        <presetDescription>4. The defined process objectives.</presetDescription>
        <customisedDescription>4. The defined process objectives.</customisedDescription>
        <preRequisiteType>PROCESS_RELATED</preRequisiteType>
      - <sources>
        - <internalSourcesList xsi:type="internalSource" sourceType="InternalSource">
            <sourceElementPath> [Process] -> [Phases] -> [Objectives Definition] ->
              Reporting</sourceElementPath>
          </internalSourcesList>
        </sources>
        <required>false</required>
        <customised>true</customised>
      </preRequisitesList>
    - <preRequisitesList version="1" xsi:type="preRequisite">
        <dateTime>Wed Mar 21 18:10:38 GMT 2012</dateTime>
        <presetDescription>5. The aims of the study and their relationship with the goals of the metabolomics
          investigation and its hypotheses and assumptions.</presetDescription>
        <customisedDescription>5. The aims of the study and their relationship with the goals of the metabolomics
          investigation and its hypotheses and assumptions.</customisedDescription>
        <preRequisiteType>STUDY_RELATED</preRequisiteType>
      - <sources>
        - <externalSourcesList xsi:type="externalSource" sourceType="ExternalSource">
            <description>Scott, I. M., C. P. Vermeer, et al. (2010). "Enhancement of Plant Metabolite Fingerprinting
              by Machine Learning." Plant Physiology 153(4): 1506-1520.</description>
            <url>http://www.plantphysiol.org/content/153/4/1506.abstract</url>
          </externalSourcesList>
        - <externalSourcesList xsi:type="externalSource" sourceType="ExternalSource">
            <description>BaniMustafa, A. (2012). A Knowledge Discovery and Data Mining Process Model for
              Metabolomics. PhD, University of Wales, Aberystwyth.</description>
            <url>file:/E:/PhD/PhD/PhDThesis/PhDThesisWriting/PhDThesisLatex/PhDLatex/PhDThesis.pdf</url>
```

```
      </externalSourcesList>
    - <externalSourcesList xsi:type="externalSource" sourceType="ExternalSource">
          <description>lynn Presentation about the experimental design of HiMet Project</description>
          <url>file:/E:/PhD/PhD/PhDThesis/PhDApplication/Application_Data/Plant_York_LC-
            MS_TargetAnalisis/Description/lynne.pdf</url>
      </externalSourcesList>
    </sources>
    <required>false</required>
    <customised>true</customised>
  </preRequisitesList>
- <preRequisitesList version="1" xsi:type="preRequisite">
    <dateTime>Wed Mar 21 18:10:38 GMT 2012</dateTime>
    <presetDescription>6. Background information and/or knowledge regarding the data mining, including: its
      approaches (see section 3.2), goals, tasks (see section 3.3), and techniques (see section
      3.4).</presetDescription>
    <customisedDescription>6. Background information and/or knowledge regarding the data mining, including: its
      approaches (see section 3.2), goals, tasks (see section 3.3), and techniques (see section
      3.4).</customisedDescription>
    <preRequisiteType>LITERATURE_RELATED</preRequisiteType>
  - <sources>
    - <externalSourcesList xsi:type="externalSource" sourceType="ExternalSource">
          <description>BaniMustafa, A. (2012). A Knowledge Discovery and Data Mining Process Model for
            Metabolomics. PhD, University of Wales, Aberystwyth.</description>
          <url>file:/E:/PhD/PhD/PhDThesis/PhDThesisWriting/PhDThesisLatex/PhDLatex/PhDThesis.pdf</url>
      </externalSourcesList>
    </sources>
    <required>false</required>
    <customised>true</customised>
  </preRequisitesList>
- <preRequisitesList version="1" xsi:type="preRequisite">
    <dateTime>Wed Mar 21 18:10:38 GMT 2012</dateTime>
    <presetDescription>7. Background information regarding the requirements of data mining techniques application,
      including: time, cost, and expertise as well as the availability of the software and hardware
      infrastructure.</presetDescription>
    <customisedDescription>7. Background information regarding the requirements of data mining techniques
      application, including: time, cost, and expertise as well as the availability of the software and hardware
      infrastructure.</customisedDescription>
    <preRequisiteType>LITERATURE_RELATED</preRequisiteType>
  - <sources>
    - <externalSourcesList xsi:type="externalSource" sourceType="ExternalSource">
          <description>BaniMustafa, A. (2012). A Knowledge Discovery and Data Mining Process Model for
            Metabolomics. PhD, University of Wales, Aberystwyth.</description>
          <url>file:/E:/PhD/PhD/PhDThesis/PhDThesisWriting/PhDThesisLatex/PhDLatex/PhDThesis.pdf</url>
      </externalSourcesList>
    </sources>
    <required>false</required>
    <customised>true</customised>
  </preRequisitesList>
</preRequisites>
+ <objectives version="1">
+ <planning version="1">
+ <performing version="1">
+ <reporting version="1">
+ <result version="1">
  <actors/>
</phase>
```
