# Supplementary material for: Computer-Aided Data Mining: Automating a Novel Knowledge Discovery and Data Mining Process Model for Metabolomics
Source: arXiv:1907.04318 source file (2019-07-09)
Supplement: Supplementary file 5 [file selectionjustification.pdf]

```
<?xml version="1.0" encoding="UTF-8" standalone="true"?>
<modelingTechniqueSelection xsi:noNamespaceSchemaLocation="" version="1" xmlns:xsi="http://www.w3.org/2001/XMLSchema-instance">
    <dateTime>Tue Mar 13 12:23:44 GMT 2012</dateTime>
    <location>E:\PhD\PhD\PhDThesis\PhDApplication\HiMet9IP_Application\HiMet9IP_11\Process\Iteration 1\Phases\4- Technique
      Selection\Iteration 1\Delivery</location>
    <technique>Artificail Nural Networks (ANN)</technique>
    <algorithm>Weka implemntation of Multilayer perceptron (MLP)</algorithm>
    <supervised>true</supervised>
    <dataMiningApproach>DATA_DRIVEN</dataMiningApproach>
    <dataMiningGoal>DISCOVERY</dataMiningGoal>
    <dataMiningTask>Classification</dataMiningTask>
    <selectionJustification>The selected technique achieve the selected objectives and suites the nature and quality of the data</selectionJustification>
  - <traceability>
    - <externalSourcesList sourceType="ExternalSource" xsi:type="externalSource">
          <description>Maimon, O. and L. Rokach (2005). Data Mining and Knowledge Discovery Handbook. New York, NY,
            Springer.</description>
      </externalSourcesList>
    - <externalSourcesList sourceType="ExternalSource" xsi:type="externalSource">
          <description>BaniMustafa, A. H. and N. W. Hardy (2012). A Strategy for Selecting Data Mining Techniques in Metabolomics (in
            press). Plant Metabolomics: Methods and Protocols. N. W. Hardy and R. D. Hall, Springer Science. 860: 317-335.</description>
      </externalSourcesList>
    - <externalSourcesList sourceType="ExternalSource" xsi:type="externalSource">
          <description>BaniMustafa, A. (2012). A Knowledge Discovery and Data Mining Process Model for Metabolomics. PhD, University of
            Wales, Aberystwyth.</description>
          <url>file:/E:/PhD/PhD/PhDThesis/PhDThesisWriting/PhDThesisLatex/PhDLatex/PhDThesis.pdf</url>
      </externalSourcesList>
    - <internalSourcesList sourceType="InternalSource" xsi:type="internalSource">
          <sourceElementPath> [Process] -> [Inputs] -> [Metabolomics Data] -> Data Set</sourceElementPath>
      </internalSourcesList>
    </traceability>
  - <measurability>
        <booleanMeasuresList xsi:type="booleanMeasure" measureType="BOOLEAN" name="Model Fitness" criteria="Is the model fit?"/>
        <booleanMeasuresList xsi:type="booleanMeasure" measureType="BOOLEAN" name="Model Under Fitness" criteria="Is the model
          underfit?"/>
        <booleanMeasuresList xsi:type="booleanMeasure" measureType="BOOLEAN" name="Model Performance" criteria="Is the model
          performance acceptable?"/>
        <quantitativeMeasuresList xsi:type="quantitativeMeasure" measureType="QUANTITATIVE" name="Correctly Classified Percentage"
          maximum="100.0" minimum="0.0" unit="percentage"/>
        <quantitativeMeasuresList xsi:type="quantitativeMeasure" measureType="QUANTITATIVE" name="Incorrectly Classified
          Percentage" maximum="100.0" minimum="0.0" unit="percentage"/>
        <quantitativeMeasuresList xsi:type="quantitativeMeasure" measureType="QUANTITATIVE" name="Correctly Classified Count"
          maximum="INF" minimum="0.0" unit="count"/>
        <quantitativeMeasuresList xsi:type="quantitativeMeasure" measureType="QUANTITATIVE" name="Incorrectly Classified Count"
          maximum="INF" minimum="0.0" unit="count"/>
        <quantitativeMeasuresList xsi:type="quantitativeMeasure" measureType="QUANTITATIVE" name="Kappa" maximum="100.0"
          minimum="0.0" unit="real number"/>
        <quantitativeMeasuresList xsi:type="quantitativeMeasure" measureType="QUANTITATIVE" name="Error Rate" maximum="100.0"
          minimum="0.0" unit="percentage"/>
        <quantitativeMeasuresList xsi:type="quantitativeMeasure" measureType="QUANTITATIVE" name="Mean Absolute Error"
          maximum="1.0" minimum="0.0" unit="real number"/>
        <quantitativeMeasuresList xsi:type="quantitativeMeasure" measureType="QUANTITATIVE" name="Mean Prior Absolute Error"
          maximum="1.0" minimum="0.0" unit="real number"/>
        <quantitativeMeasuresList xsi:type="quantitativeMeasure" measureType="QUANTITATIVE" name="Relative Absolute Error"
          maximum="100.0" minimum="0.0" unit="real number"/>
        <quantitativeMeasuresList xsi:type="quantitativeMeasure" measureType="QUANTITATIVE" name="Root Mean Squared Error"
          maximum="1.0" minimum="0.0" unit="real number"/>
        <quantitativeMeasuresList xsi:type="quantitativeMeasure" measureType="QUANTITATIVE" name="Root Mean Prior Squared Error"
          maximum="1.0" minimum="0.0" unit="real number"/>
        <quantitativeMeasuresList xsi:type="quantitativeMeasure" measureType="QUANTITATIVE" name="Root Relative Squared Error"
          maximum="100.0" minimum="0.0" unit="real number"/>
        <otherMeasuresList xsi:type="measure" measureType="OTHER" name="Confusion Matrix"/>
        <otherMeasuresList xsi:type="measure" measureType="OTHER" name="Classification Details"/>
    </measurability>
  - <feasibility>
        <requiredTime>2.0</requiredTime>
        <feasible>true</feasible>
    </feasibility>
```

```
- <successCriteria>
      <description>The model should be able to correctly classify unknown samples of data.</description>
  - <expectedOutcomes>
    - <resultsList>
          <measure xsi:type="booleanMeasure" measureType="BOOLEAN" name="Model Fitness" criteria="Is the model fit?"/>
          <outcome result="true"/>
      </resultsList>
    - <resultsList>
          <measure xsi:type="booleanMeasure" measureType="BOOLEAN" name="Model Under Fitness" criteria="Is the model
            underfit?"/>
          <outcome result="false"/>
      </resultsList>
    - <resultsList>
          <measure xsi:type="booleanMeasure" measureType="BOOLEAN" name="Model Performance" criteria="Is the model
            performance acceptable?"/>
          <outcome result="false"/>
      </resultsList>
    - <resultsList>
          <measure xsi:type="quantitativeMeasure" measureType="QUANTITATIVE" name="Correctly Classified Percentage"
            maximum="100.0" minimum="0.0" unit="percentage"/>
          <outcome result="60.0"/>
      </resultsList>
    - <resultsList>
          <measure xsi:type="quantitativeMeasure" measureType="QUANTITATIVE" name="Incorrectly Classified Percentage"
            maximum="100.0" minimum="0.0" unit="percentage"/>
          <outcome result="40.0"/>
      </resultsList>
    - <resultsList>
          <measure xsi:type="quantitativeMeasure" measureType="QUANTITATIVE" name="Error Rate" maximum="100.0"
            minimum="0.0" unit="percentage"/>
          <outcome result="40.0"/>
      </resultsList>
    - <resultsList>
          <measure measureType="OTHER" name="Confusion Matrix"/>
          <outcome result="correctly calssified examples must be over 50% across all classed"/>
      </resultsList>
    - <resultsList>
          <measure measureType="OTHER" name="Classification Details"/>
          <outcome result="godd classification performance"/>
      </resultsList>
    </expectedOutcomes>
  </successCriteria>
- <acheivability>
      <suitableForDataNature>true</suitableForDataNature>
      <suitableForDataTypes>true</suitableForDataTypes>
      <suitableForDataSize>true</suitableForDataSize>
      <suitableForDataQuality>true</suitableForDataQuality>
      <suitableForDataDistribution>true</suitableForDataDistribution>
      <acheivingObjectives>true</acheivingObjectives>
      <requirmentsAvailable>true</requirmentsAvailable>
      <requireIntensiveAcclimatisation>true</requireIntensiveAcclimatisation>
  </acheivability>
   <finalSelection>true</finalSelection>
</modelingTechniqueSelection>
```
