# Supplementary material for: Computer-Aided Data Mining: Automating a Novel Knowledge Discovery and Data Mining Process Model for Metabolomics
Source: arXiv:1907.04318 source file (2019-07-09)
Supplement: Supplementary file 6 [file study.pdf]

```
<?xml version="1.0" encoding="UTF-8" standalone="true"?>
<project xsi:noNamespaceSchemaLocation="" name="HiMet9IP_1" xmlns:xsi="http://www.w3.org/2001/XMLSchema-instance">
    <location>E:\PhD\PhD\PhDThesis\PhDApplication\HiMet9IP_Application</location>
    <date>Tue Mar 13 13:30:35 GMT 2012</date>
    <description/>
  - <inputs>
    - <metabolomicsData version="1" isExternal="false">
          <dateTime>Tue Mar 20 15:14:24 GMT 2012</dateTime>
      + <prospecting version="1">
      + <understanding version="1">
      + <dataSet version="1" isExternal="false">
      + <metaData version="1" isExternal="false">
      </metabolomicsData>
    - <metabolomicsStudy version="1">
          <dateTime>Tue Mar 13 12:23:43 GMT 2012</dateTime>
          <metabolomicsApproach>TARGET_ANALYSIS</metabolomicsApproach>
          <aims>Testing the discrimination between arabidopsis thaliana genotypes using samples from the plant leaf
             extracts.</aims>
      - <investigation>
            <question>Can the mutation of Arabidopsis Thaliana be monitored using metabolmics data.</question>
            <goal>Applying metabolomics in plant genetics</goal>
        </investigation>
      - <assay>
        - <sample>
              <bioSource>Arabidopsis Thaliana</bioSource>
              <SampleType>Leaf Extract</SampleType>
              <growthProtocols>The Arabidopsis plants were grown and harvested by the HiMet project
                 collaborators in The John Innes Centre(JIC), where the samples growth, harvest, extraction and
                 preparation protocols were collected and recorded as meta-data in compliance with ArMet
                 model. The plants were grown using 9 blocks under a temperature of 18-23 c, with 70\%
                 relative humidity and 16 hours of day light.</growthProtocols>
              <harvestProtocols>The harvesting protocols involved collecting aerial tissues from the mutant
                 plants. The samples metabolism were then quenched using liquid $N_{2}$ in mid light and then
                 freezed, dried, and powdered. They were then shipped in a few days at ambient temperature,
                 where the storage temperature was -80\textcelsius.</harvestProtocols>
              <standards>alpha-tocopherol</standards>
              <SamplePreparation>The samples were based on fractions of the chlorform layer extracted from the
                 plants leaf. The sample preparation was performed under a temperature of 15\textcelsius.
                 $\alpha$-tocopherol was used as an internal standard. An amount of 5mg of on ice were
                 extracted in 200 $\mu L$ of methanol during a period of 5 minutes. Then a 200 $\mu L$ of 50
                 mM Tris-HCl was added during a period of 10 minutes with a pH of 7.5. This was followed by
                 800 $\mu L$ of chloroform extract for a period of 10 minutes. The sample then centrifuged for
                 5 minutes at 3000g at 4\textcelsius. The choroform layer sample then transferred to glass vials
                 and dried down in speedvac. The precipitate then re-suspended in 50 $\mu l$ MTBE.
                 </SamplePreparation>
          </sample>
        - <instrument>
              <info>The dried layers of chloroform were analysed on a 250-mm (4.6mmi.d.) using C30 column
                 (5 $\mu m$YMC30;YMC), at a flow rate of 1 ml$min^{-1}$, with 0.2\% formic acid and
                 20mM ammonium formate in 80\%methanol, or methyl tertiary-butyl ether (solvent B) as 0\%
                 for a period of 6 minutes, 15\% for a period of 5 minutes , to 90\% for a period of 30 minutes,
                 and 90\% for a period of 5 minutes. The quantification of the isoprenoids were conducted using
                 positive-ion atmospheric pressure chemical ionisation MS using capillary at 15 V and 150
                 \textcelsius, and using a vaporiser at 500\textcelsius, and discharge current of 5 $\mu A$
                 </info>
          </instrument>
            <assayDataFormat>METABOLITE_CONCENTRATION</assayDataFormat>
            <fileFormat>.csv</fileFormat>
            <technique>LC-MS</technique>
            <runs>3</runs>
            <replica>9</replica>
```

<preProcessingProcedures>The samples were based on fractions of the chlorform layer extracted from the plants leaf. The sample preparation was performed under a temperature of 15\textcelsius. $\alpha$-tocopherol was used as an internal standard. An amount of 5mg of on ice were extracted in 200 $\mu L$ of methanol during a period of 5 minutes. Then a 200 $\mu L$ of 50 mM Tris-HCl was added during a period of 10 minutes with a pH of 7.5. This was followed by 800 $\mu L$ of chloroform extract for a period of 10 minutes. The sample then centrifuged for 5 minutes at 3000g at 4\textcelsius. The choroform layer sample then transferred to glass vials and dried down in speedvac. The precipitate then re-suspended in 50 $\mu l$ MTBE. </preProcessingProcedures>
</assay>
</metabolomicsStudy>
</inputs>
+ <sources>
+ <process version="1">
- <supplements>
+ <management>
+ <humanInteraction>
+ <standards>
+ <quality>
</supplements>
</project>
