# Supplementary material for: Computer-Aided Data Mining: Automating a Novel Knowledge Discovery and Data Mining Process Model for Metabolomics
Source: arXiv:1907.04318 source file (2019-07-09)
Supplement: Supplementary file 7 [file modelingtechniqueselection.pdf]

```

<?xml version="1.0" encoding="UTF-8" standalone="true"?>
<modelingTechniqueSelection xsi:noNamespaceSchemaLocation="" version="1"
xmlns:xsi="http://www.w3.org/2001/XMLSchema-instance">
  <dateTime>Tue Mar 13 12:23:44 GMT 2012</dateTime>
  <location>E:\PhD\PhD\PhDThesis\PhDApplication\HiMet9IP_Application\HiMet9IP_11\Process\Iteration 1
    \Phases\4- Technique Selection\Iteration 1\Delivery</location>
  <technique>Artificail Nural Networks (ANN)</technique>
  <algorithm>Weka implemntation of Multilayer perceptron (MLP)</algorithm>
  <supervised>true</supervised>
  <dataMiningApproach>DATA_DRIVEN</dataMiningApproach>
  <dataMiningGoal>DISCOVERY</dataMiningGoal>
  <dataMiningTask>Classification</dataMiningTask>
  <selectionJustification>The selected technique achieve the selected objectives and suites the nature and quality of
    the data</selectionJustification>
  - <traceability>
    - <externalSourcesList sourceType="ExternalSource" xsi:type="externalSource">
      <description>Maimon, O. and L. Rokach (2005). Data Mining and Knowledge Discovery Handbook.
        New York, NY, Springer.</description>
    </externalSourcesList>
    - <externalSourcesList sourceType="ExternalSource" xsi:type="externalSource">
      <description>BaniMustafa, A. H. and N. W. Hardy (2012). A Strategy for Selecting Data Mining
        Techniques in Metabolomics (in press). Plant Metabolomics: Methods and Protocols. N. W. Hardy
        and R. D. Hall, Springer Science. 860: 317-335.</description>
    </externalSourcesList>
    - <externalSourcesList sourceType="ExternalSource" xsi:type="externalSource">
      <description>BaniMustafa, A. (2012). A Knowledge Discovery and Data Mining Process Model for
        Metabolomics. PhD, University of Wales, Aberystwyth.</description>
      <url>file:/E:/PhD/PhD/PhDThesis/PhDThesisWriting/PhDThesisLatex/PhDLatex/PhDThesis.pdf</url>
    </externalSourcesList>
    - <internalSourcesList sourceType="InternalSource" xsi:type="internalSource">
      <sourceElementPath>[Process] -> [Inputs] -> [Metabolomics Data] -> Data Set</sourceElementPath>
    </internalSourcesList>
  </traceability>
  - <measurability>
    <booleanMeasuresList xsi:type="booleanMeasure" measureType="BOOLEAN" name="Model Fitness"
      criteria="Is the model fit?"/>
    <booleanMeasuresList xsi:type="booleanMeasure" measureType="BOOLEAN" name="Model Under
      Fitness" criteria="Is the model underfit?"/>
    <booleanMeasuresList xsi:type="booleanMeasure" measureType="BOOLEAN" name="Model
      Performance" criteria="Is the model performance acceptable?"/>
    <quantitativeMeasuresList xsi:type="quantitativeMeasure" measureType="QUANTITATIVE"
      name="Correctly Classified Percentage" maximum="100.0" minimum="0.0" unit="percentage"/>
    <quantitativeMeasuresList xsi:type="quantitativeMeasure" measureType="QUANTITATIVE"
      name="Incorrectly Classified Percentage" maximum="100.0" minimum="0.0" unit="percentage"/>
    <quantitativeMeasuresList xsi:type="quantitativeMeasure" measureType="QUANTITATIVE"
      name="Correctly Classified Count" maximum="INF" minimum="0.0" unit="count"/>
    <quantitativeMeasuresList xsi:type="quantitativeMeasure" measureType="QUANTITATIVE"
      name="Incorrectly Classified Count" maximum="INF" minimum="0.0" unit="count"/>
    <quantitativeMeasuresList xsi:type="quantitativeMeasure" measureType="QUANTITATIVE"
      name="Kappa" maximum="100.0" minimum="0.0" unit="real number"/>
    <quantitativeMeasuresList xsi:type="quantitativeMeasure" measureType="QUANTITATIVE"
      name="Error Rate" maximum="100.0" minimum="0.0" unit="percentage"/>
    <otherMeasuresList xsi:type="measure" measureType="OTHER" name="Confusion Matrix"/>
    <otherMeasuresList xsi:type="measure" measureType="OTHER" name="Classification Details"/>
  </measurability>
  - <feasibility>
    <requiredTime>2.0</requiredTime>
    <feasible>true</feasible>
  </feasibility>

```

```

- <successCriteria>
  <description>The model should be able to correctly classify unknown samples of data.</description>
- <expectedOutcomes>
  - <resultsList>
    <measure xsi:type="booleanMeasure" measureType="BOOLEAN" name="Model Fitness"
      criteria="Is the model fit?"/>
    <outcome result="true"/>
  </resultsList>
  - <resultsList>
    <measure xsi:type="booleanMeasure" measureType="BOOLEAN" name="Model Under
      Fitness" criteria="Is the model underfit?"/>
    <outcome result="false"/>
  </resultsList>
  - <resultsList>
    <measure xsi:type="booleanMeasure" measureType="BOOLEAN" name="Model
      Performance" criteria="Is the model performance acceptable?"/>
    <outcome result="false"/>
  </resultsList>
  - <resultsList>
    <measure xsi:type="quantitativeMeasure" measureType="QUANTITATIVE"
      name="Correctly Classified Percentage" maximum="100.0" minimum="0.0"
      unit="percentage"/>
    <outcome result="60.0"/>
  </resultsList>
  - <resultsList>
    <measure xsi:type="quantitativeMeasure" measureType="QUANTITATIVE"
      name="Incorrectly Classified Percentage" maximum="100.0" minimum="0.0"
      unit="percentage"/>
    <outcome result="40.0"/>
  </resultsList>
  - <resultsList>
    <measure xsi:type="quantitativeMeasure" measureType="QUANTITATIVE" name="Error
      Rate" maximum="100.0" minimum="0.0" unit="percentage"/>
    <outcome result="40.0"/>
  </resultsList>
  - <resultsList>
    <measure measureType="OTHER" name="Confusion Matrix"/>
    <outcome result="correctly calssified examples must be over 50% across all classed"/>
  </resultsList>
  - <resultsList>
    <measure measureType="OTHER" name="Classification Details"/>
    <outcome result="godd classification performance"/>
  </resultsList>
</expectedOutcomes>
</successCriteria>
- <acheivability>
  <suitableForDataNature>true</suitableForDataNature>
  <suitableForDataTypes>true</suitableForDataTypes>
  <suitableForDataSize>true</suitableForDataSize>
  <suitableForDataQuality>true</suitableForDataQuality>
  <suitableForDataDistribution>true</suitableForDataDistribution>
  <acheivingObjectives>true</acheivingObjectives>
  <requirmentsAvailable>true</requirmentsAvailable>
  <requireIntensiveAcclimatisation>true</requireIntensiveAcclimatisation>
</acheivability>
  <finalSelection>true</finalSelection>
</modelingTechniqueSelection>

```
